# Supplementary material for: InFusion: Inpainting 3D Gaussians via Learning Depth Completion from Diffusion Prior
Source: arXiv:2404.11613 source file (2024-04-17)
Supplement: Supplementary file 1 [file 7.appendix.tex]

\clearpage
\appendix

\setcounter{figure}{0}
\setcounter{table}{0}
\setcounter{equation}{0}

\section*{Appendix}

\section{Overview}\label{appendix:overview}

Overview of the appendix.
